# Supplementary material for: How moving cracks in brittle solids choose their path
Source: arXiv:2004.03115 ancillary file (2020-09-10)
Supplement: Supplementary file 1 [file SI_path_selection_4.pdf]

# Supplementary Material for: How moving cracks in brittle solids choose their path

Lital Rozen-Levy,[1] John M. Kolinski,[2] Gil Cohen,[1] and Jay Fineberg[1]

[1]*The Racah Institute of Physics, The Hebrew University of Jerusalem, Givat Ram, Jerusalem Israel*

[2]*École Polytechnique Fédérale de Lausanne, 1015 Lausanne, Switzerland*

(Dated: August 10, 2020)

## MATERIALS AND METHODS

### Materials

To prepare samples of polyacrylamide hydrogels with embedded polyamide particles, we begin with a solution of unpolymerized polyacrylamide monomer with a small amount of bis-acrylamide cross linker (Sigma Aldrich). We used a total monomer concentration of 13.7% (wt) with 2.7% (wt) cross-linker. Polymerization is initiated and catalyzed with 0.2% Ammonium per sulfate (APS) and 0.02 % Tetramethylethylenediamine (TEMED). Polymerization takes place in a temperature conditioned laboratory at 19 C for four hours prior to experiments. As prepared, this gel has an elastic modulus of approximately 90 kPa, a longitudinal wave velocity of approximately 11 m/sec, a shear wave velocity of approximately 5.5 m/sec and, as the material is incompressible, its Poisson's ratio is 0.5 and thus the Rayleigh wave speed is calculated to be 5.3 m/sec[1]. We add a small concentration of polyamide particles having an average diameter of 50 microns and a stiffness of several GPa (Dantec dynamics). With this elastic modulus, the particles can be considered to be 'infinitely rigid' relative to the gels. Particles were mixed at a numerical density in the gel sample of approximately 1-3 particles per 200 picoliter, or an average area density of 1 - 3 particle per $mm^2$ for a 190 micron thick gel. The crack tips analyzed had, typically, densities of 2 - 6 particles per $mm^2$.

Gel samples were cast between two glass plates separated by 190-micron spacers. On the surface of one glass plate, a grid is embossed with a lateral spacing of 60 microns; this imprints the undeformed reference state of the gel upon its surface.

## Methods

All calculations and analysis are performed in the 'reference' (undistorted) frame. Purely tensile loads are applied in the vertical ($y$-direction) boundaries of the gel samples by rigid displacement of two grips. To one grip a load cell is attached, whose voltage is amplified by a lock-in amplifier, enabling precise measurement of the applied load. The other grip is attached to a precision displacement stage that applies remote tensile strain to the gel sample. The $x$ direction is defined as the direction normal to that of the applied tensile strain. For the samples used to study crack-particle interactions, the $x$ x $y$ sample dimensions were 60 x 40 mm, whereas for the oscillatory instability, sample sizes of 200 x 200 mm were used. The center 10 x 6mm section of each sample was illuminated normal to its surface, and imaged onto a fast camera's sensor (IDT Y7 S3) at 8000 fps, as shown schematically in Fig. 1 (a). Each of the 2000 x 1000 pixels of the camera was mapped to 6 microns x 6 microns. The mean accelerations and velocities of the cracks were controlled by the pre-imposed strain as described elsewhere[2]. In the strip samples, the applied strain varied from 10 – 25%. For the oscillatory experiments, strains of about 10% were used. After each sample was stretched to the desired strain, a notch, typically 1 mm in length, was inserted into the middle of the sample's edge using a scalpel. Upon cutting the notch, the crack begins to propagate, as shown in Fig. 1 (b). As the crack propagates through the sample, the load measured by the load cell falls; this monotonically decreasing signal was used to trigger the acquisition of images in the fast camera's circular buffer. The images are stored for post-processing.

The strain field is measured by means of distortions of a reference grid embossed on the sample's surface, using a precision stamp fabricated using photolithography. The grid has a depth of 2 microns and the grid squares are 60 microns along a side. The displacement of each grid location is measured by determining the distances between adjacent grid points in the laboratory frame, and comparing this to the grid's unstressed dimensions in the reference frame. The location of each grid point is determined to sub-pixel resolution by fitting a spline interpolated path through up to 10 neighboring grid points in each row and column. The error in locating each grid point is 1/3 of a pixel. We calculate the deformation fields using finite differences of neighboring grid displacements. These derivatives are then used to calculate the 2-D deformation gradient tensor, $F_{ij} = \partial_i u_j$. Typical results of this

post-processing are shown for a homogeneous sample and a sample with a particle near the crack tip in Fig. 1 (b) and (c), respectively.

The crack tip location is determined in each image first by applying a canny edge filter to identify the entire crack tip opening displacement. The pixel furthest in the direction of the crack's advancement is designated as the crack tip in the image. The crack tip thus identified delineates the region within the gel where the surfaces start to separate. The error in identifying the crack tip is bound by the pixel size (6 microns) and the process zone scale (20 microns[4])) along the $x$-axis, and is only 6 microns along the $y$-axis. We take advantage of the better-resolved data away from the crack tip to construct an interpolation function for the grid location data, and either interpolate or extrapolate to find the crack tip location in the grid coordinate system. Our maximum error in locating the crack tip is approximately 1/3 of the grid spacing.

The Strain Energy Density (SED) was determined directly from the deformation fields. The analysis is confined to a region of approximately 1 $mm^2$ ahead of the propagating crack (in the reference frame), where values outside of a 120 degree arc along the crack's path were not used for the predictors. For the hydrogels considered here, this scale exceeds the weakly nonlinear scale at which the linear elastic description breaks down[3]. For these materials, the nonlinear scale increases as the crack speed increases. It is typically about 100 microns (about two grid spacings) from the crack tip[4]. The process zone is much smaller, at most 20 microns in size[4]. Thus, the range analyzed (7-10 grid spacings) is the scale where LEFM nominally applies; nevertheless, we use the neo-Hookean strain energy density to account for finite deformation in the near-tip region. The strain energy density, $U$, is calculated via $U(F) = \frac{\mu}{2}\left[F_{ij}F_{ij} + \lambda^2 - 3\right]$, where $\lambda = \det(F)^{-1}$, and $\mu$ is the gel's shear modulus[5, 6]. To develop a prediction of the crack's path, the instantaneous $U(x, y)$ is evaluated near the crack tip within a 120 degree acceptance angle, $\pm 60$ from the crack's propagation axis, ahead of the crack tip.

The crack's direction is determined by the relative position of the sequential crack tip location. The sequential crack tip location is mapped back from the laboratory frame into the reference frame by counting grid spacings, using the grid corresponding to the current image. Along each column between the current and next crack tip locations, the maximum of $U$ is found. The location of the maximum of $U$ for each $x$ was determined by fitting a parabola through the measured $U(y)$ data using the $\pm 3$ grid points neighboring the measured maximal

value of $U$. This procedure resulted in a resolution of approximately 0.4 grid spacings. The SED predictor was then determined via a linear fit of the maximal locations of $U$; its slope yielded the predicted angles in Figs. 3-5. Using this procedure we reduced the measurement error for the SED predictors to less than 2 degrees, or approximately one third of the size of the data points plotted in Fig. 5.

Imaging artifacts can arise in our experimental system from a number of different sources, and these ultimately lead to the regions near the crack tip where the strains are ill-defined (whited out regions). Such regions are not included in our analysis. These ill-defined regions result from the strong slopes of the sample surfaces at the crack tip. This caused the imaging plane and the grid plane to be misaligned in this region. The strong sample curvature near the crack tip additionally gave rise to lensing leading to the dark or light regions in the images recorded by the fast camera's imaging sensor. With repeated use, the embossing grid becomes damaged. This damage is typically local, and readily identifiable in an image sequence. Damaged regions of the grid stamp show up as light or dark regions on the image depending on the relative alignment of the focal- and grid planes, as can be observed, for example, in Fig. 1 (c).

## THE INFLUENCE OF RIGID PARTICLES ON THE SURROUNDING GEL

The interaction of a propagating crack with a rigid inclusion, as explored in the main manuscript, is mediated by the elastic fields. Indeed, it is only via perturbations to the elastic field that the crack tip 'knows' that the rigid inclusion is present. The particles have a density very near to that of the gel, and their effect on the inertia of the material is essentially negligible. Their main effect is to alter the boundary conditions imposed throughout the sample by pinning the material at each particle's boundary. The elastic material at the particle boundaries is therefore constrained to be displacement-free.

The presence of rigid particles clearly alters the strain fields. We evaluate the effect of isolated particles on the strain fields surrounding a propagating crack in Fig. S1. Over a period of 0.25 msec, the crack's path is significantly altered due to the presence of the particles. This has direct consequences on the form of the strain field near the crack tip, which, in homogeneous materials, is singular [7, 8]. The typically large distortions of the unperturbed deformation fields that take place once a crack tip approaches a particle can be

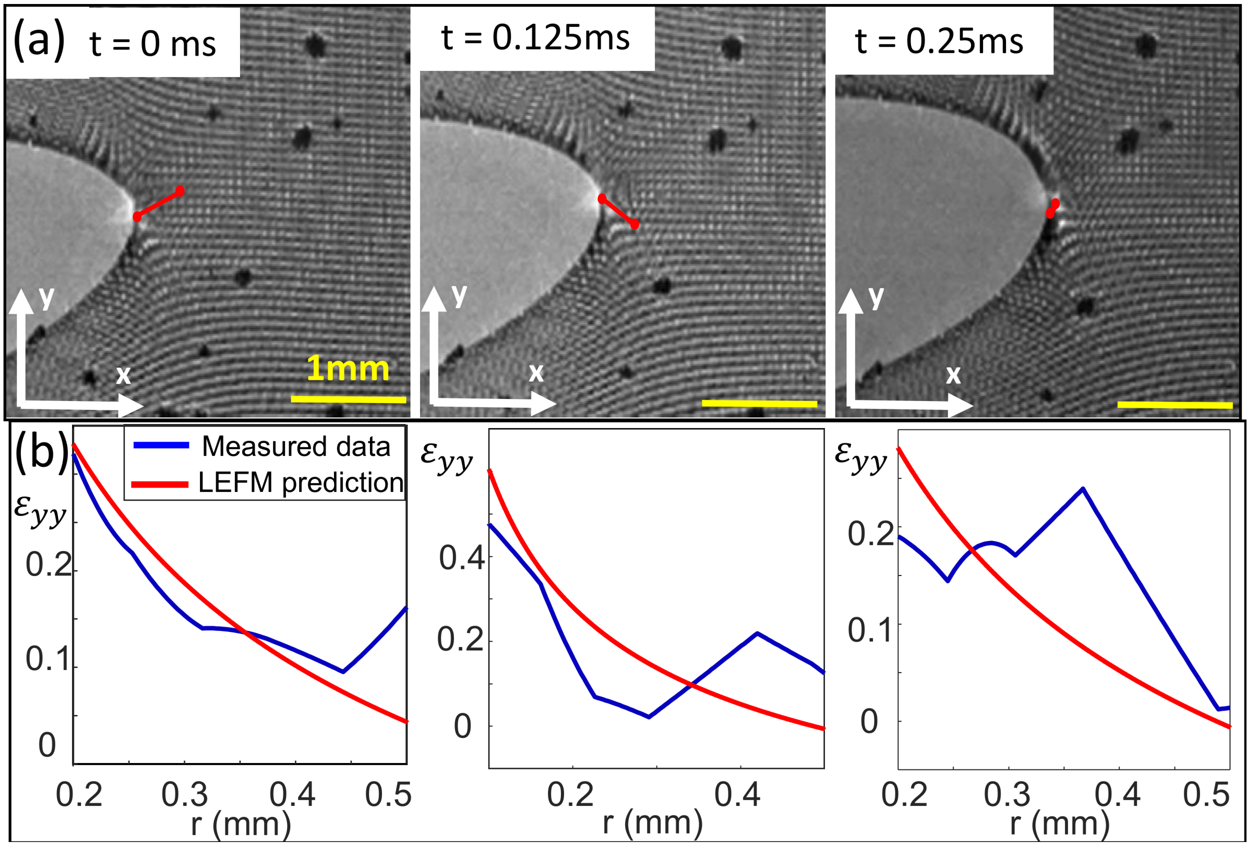


Fig. S 1. The elastic fields surrounding a crack tip rapidly evolve as the crack interacts with particles that it encounters. (a) A typical time series of images of a crack moving at $v = 0.3c_R$, separated by 0.125 msec intervals. Red lines delineate the crack's trajectory. (b) $\epsilon_{yy}$ along the crack trajectory directions are represented in blue. The corresponding LEFM predictions are noted by the red lines. At $t = 0$ msec the particles are far from the tip, so $\epsilon_{yy}$ is close to the LEFM prediction. As the crack tip approaches the particles, at $t = 0.125$ msec and at $t = 0.25$ msec, $\epsilon_{yy}$ becomes increasingly distorted. By $t = 0.25$ msec the $\epsilon_{yy}$ fields are distorted by nearly 100% relative to the particle-free fields.

readily seen from the comparison of the measured deformations and the LEFM predictions for the strain, as shown in Fig. S1 (b).

The elastic deformations are directly measured in the material frame of reference by the grid that is embossed on the surface of the sample, as described in the main text and elsewhere [8, 9]. In Fig. S2 (a) we highlight two regions with circles that are symmetrically located on both sides of a crack's trajectory. The corresponding measured strain component within approximately 1 mm of the crack tip, $\epsilon_{yy} = \partial_y u_y$, is presented in Fig. S2 (b). The

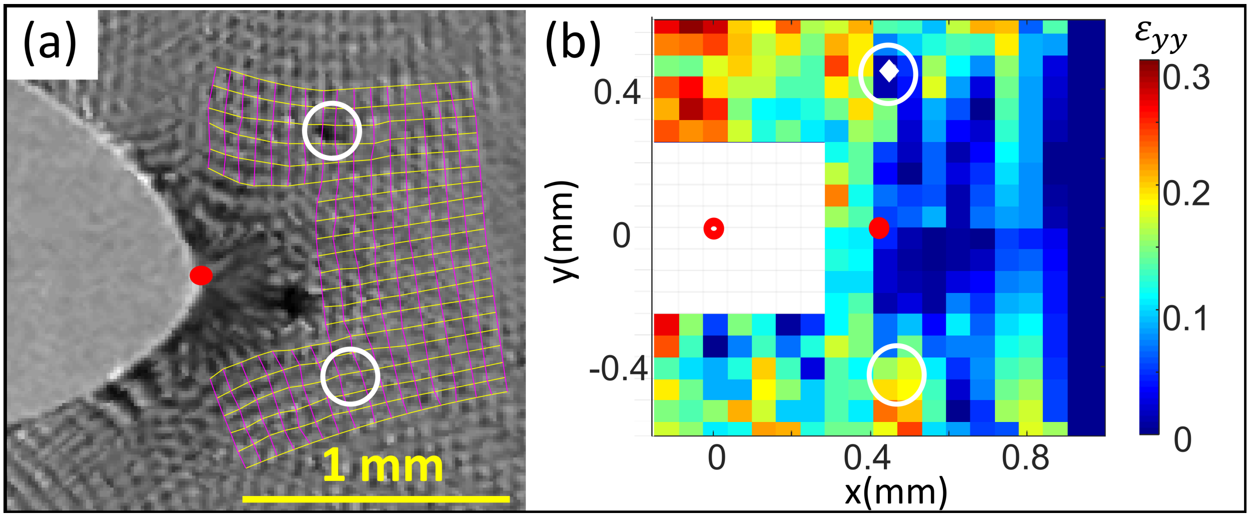


Fig. S 2. The influence of external particles embedded within the gel. (a) A typical sample image, the red point denotes the crack tip, the detected grids are overlayed in color on the image, and the circled area above the crack tip includes a single particle. One can see that gel has rigidly adhered to the particle's boundaries preventing it from stretching and distorting the grid. This is in clear contrast, to the symmetric location (lower circled area) below the crack tip that does not contain a particle. Here, the grid shows considerable material distortion. (b) The strain component, $\epsilon_{yy} = \partial_y u_y$, of the image in a). Clearly, the area near the particle (white diamond) did not stretch, in comparison to the (lower circle) symmetric area.

upper circle contains an isolated particle. There, the $\epsilon_{yy}$ field indicates zero-strain around the particle. In contrast, within the lower circle that does not contain a particle, the strain is indeed substantial, approaching 25%.

## LOCAL SYMMETRY ANALYSIS AT MESOSCOPIC SCALES

The characteristic parabolic form of crack tip away from the near-tip region (Fig. S3 a & b) suggests that, on average, the singular fields are retained at spatial scales that are much larger than the spacing between inhomogeneities, but still small enough that they are within the cone of influence of longitudinal waves emitted from the crack tip. At these scales, the observed mean path deviations are quite small; Indeed, the symmetry axis of the CTOD typically persists within a few degrees from one frame to the next. In addition, the energy release rate described by the CTOD curvature at these scales is wholly consistent with the

measured fracture energy, as confirmed by prior measurements [8].

The direction of propagation predicted by the local symmetry of the strain field near the crack tip, in fact, corresponds quite well to the change of the orientation of the symmetry axis as measured from the parabolic CTOD form away from the crack tip, as demonstrated in Fig. S3 c). Here, we measure the normalized eigenvectors of the strain linearized strain tensor ($\epsilon_{ij} = 1/2\,(\partial u_{i,j} + \partial u_{j,i})$) in the near-field. A prediction from this field is formed by diagonalizing $\epsilon_{ij}$ in the approximate 0.25 mm$^2$ region immediately ahead of the crack tip, where the strain data are defined. This typically consists of 49-100 grid locations. For each point in this set of grid data, we determine the direction of maximal strain. The values of the LS predictor are then calculated by averaging the values of the directions normal to the maximal strains. The error in this prediction is defined by the standard error of the sample mean, and is typically less than one degree.

The central consequence of this work is the very general result that a crack's propagation direction at the near-tip ('local') scale is guided by the SED criterion. We have seen that this criterion works extremely well for highly dynamic cracks in diverse situations, from a well-established singularity at the crack's tip, to a nearly entirely blunted crack tip.

While the SED criterion is distinct from the principle of maximum energy release rate, in that it reflects an instantaneous measurement of the strain energy density rather than the energy dissipation rate, it appears to capture the important features of the maximum energy release rate criterion, especially in the near field where we evaluate the SED.

The principle of local symmetry is recovered at larger (mesoscopic $\sim$ 1mm) scales when the crack is unperturbed by particles in the near-tip field, and its path is, on average, straight. As the PLS only applies for singular crack fields, this is consistent with our observation that the LS criterion fails to predict crack paths in the absence of the singular field, as occurs when particles are in the very near field. Indeed, for cracks with an approximate singularity in place, we observe good agreement between the large-scale symmetry of the CTOD and the LS used to evaluate path selection throughout this study, as shown in Fig. S3. For a singular field, the LS fully agrees with the classical definition of the PLS – the shear loading at the crack tip is zero.

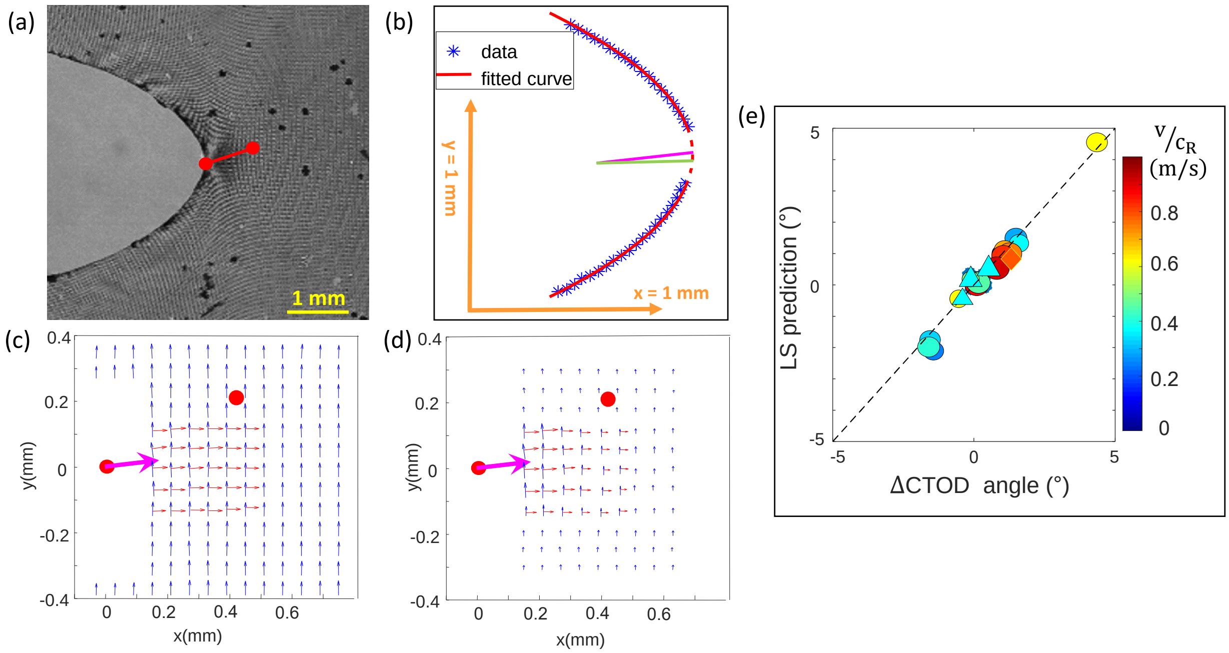


Fig. S 3. Comparison of ΔCTOD predictor with the LS criterion evaluated from the eigenvectors of the linearized strain tensor in the near-tip field. a) A crack propagates through the gel with tip location at the red dot. The red line and second red dot indicate the crack tip location in the following frame. b) The CTOD is measured from the image in (a). Blue asterisks are the CTOD data and the red line a parabolic fit. Axes are in the laboratory frame of reference. The dashes at the tip correspond to the near-tip region not included in the fit. The symmetry axis of the fitted parabola is denoted by the green line; the symmetry axis from the following frame is shown in pink. c) The normalized eigenvectors of $\epsilon_{ij}$ are plotted in the grid-frame of reference in the $\sim$0.25 mm$^2$ region ahead of the crack tip. The red arrows are orthogonal to the largest eigenvectors. Their average orientation is the LS predictor, plotted by the pink arrow. This direction is oriented at $\sim$ 1 degree from the $x$-axis. The red point indicates the location of the crack tip in the following frame; notably, the LS predictor does not agree with the near-field direction taken by the crack, which corresponds well to the SED predictor. (d) Unnormalized eigenvectors of the $\epsilon_{ij}$ presented in (c). In contrast to (c), both principle eigenvectors are shown. e) The LS predictors for over 20 experiments at $0.1 < v/c_R < 0.9$ are plotted against the change in orientation of the symmetry axis of the CTOD, ΔCTOD. The excellent agreement suggests that, at mesoscopic scales, the local symmetry criterion predicts the mesoscopic crack direction. Orange diamond: data from (a)-(c).

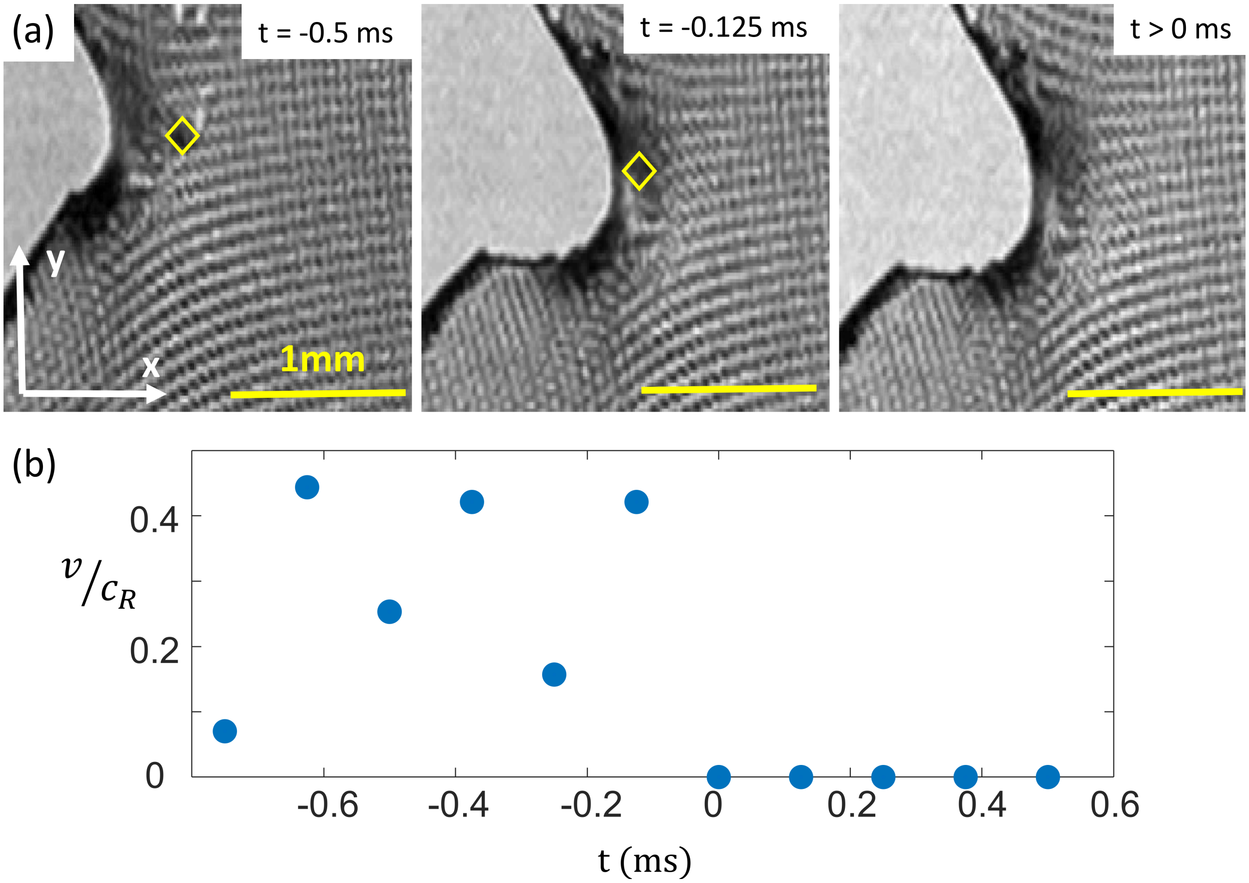


Fig. S 4. Crack arrest caused by a crack interaction with an isolated particle. (a) A series of photographs in which a crack approaches an isolated particle (highlighted by a yellow diamond). (b) The crack's instantaneous velocity as a function of time. Note that beyond t=0 the crack has entirely arrested.

## DYNAMIC CRACK ARREST RESULTING FROM A CRACK'S INTERACTION WITH A SINGLE PARTICLE

The effect of rigid particles on a propagating crack can have macroscopic consequences, despite the very local nature of the perturbation. Depending on a crack's velocity and the configuration of the particles relative to the crack tip, a crack can entirely arrest, even when there is sufficient elastic energy available to enable the crack's rapid propagation. A typical such example is depicted in Fig. S4. The crack shown propagated at velocities up to $0.4c_R$ as it approached an isolated particle. Once encountering the particle, the crack immediately arrested.

[1] A. Livne, G. Cohen, and J. Fineberg, Universality and Hysteretic Dynamics in Rapid Fracture, Phys. Rev. Lett. **94**, 224301 (2005).

[2] T. Goldman, A. Livne, and J. Fineberg, Acquisition of Inertia by a Moving Crack, Phys. Rev. Lett. **104**, 114301 (2010).

[3] E. Bouchbinder, A. Livne, and J. Fineberg, Weakly Nonlinear Theory of Dynamic Fracture, Phys. Rev. Lett. **101**, 10.1103/PhysRevLett.101.264302 (2008).

[4] A. Livne, E. Bouchbinder, I. Svetlizky, and J. Fineberg, The Near-Tip Fields of Fast Cracks, Science **327**, 1359 (2010).

[5] J. K. Knowles and E. Sternberg, Large deformations near a tip of an interface-crack between two Neo-Hookean sheets, J Elasticity **13**, 257 (1983).

[6] E. Bouchbinder, A. Livne, and J. Fineberg, The 1/r singularity in weakly nonlinear fracture mechanics, J. Mech. Phys. Solids **57**, 1568 (2009).

[7] E. Bouchbinder, Dynamic Crack Tip Equation of Motion: High-Speed Oscillatory Instability, Phys. Rev. Lett. **103**, 164301 (2009).

[8] T. G. Boué, G. Cohen, and J. Fineberg, Origin of the Microbranching Instability in Rapid Cracks, Phys. Rev. Lett. **114**, 054301 (2015).

[9] T. Goldman, R. Harpaz, E. Bouchbinder, and J. Fineberg, Intrinsic Nonlinear Scale Governs Oscillations in Rapid Fracture, Phys. Rev. Lett. **108**, 104303 (2012).
